# Supplementary material for: Hierarchical Planning and Control for Box Loco-Manipulation
Source: arXiv:2306.09532 source file (2023-07-08)
Supplement: Supplementary file 1 [file additional.tex]

\section{Additional Results}

\subsection{Chest Juggling}

We also create a chest juggling skill, where the chest of the character is used to receive and bounce the ball. See Fig.~\ref{fig:teaser} for visualization.

\subsection{Foot Stalling}

Another common soccer juggling skill is foot stalling. To create a foot stalling skill, we create an additional control node called Right Foot Stall, or RFS. In the right foot stall, the reference motion is a fixed pose with the character standing on the left leg with the right leg lifted up, and the soccer ball lying still on top of the right foot. Directed edges from RFD to RFS and RFS to RFU are created to indicate transitions between them. To generate foot stalling motion with appropriate length, another edge connecting RFS to itself is also created. The weight of this self connected edge is set to be $30$ to indicate a desired longer duration of the stalling motion. See Fig.~\ref{fig:stall} for the control graph for generating a foot stall policy.

\begin{figure}
    \centering
    \includegraphics[width=0.5\columnwidth]{figures/stall.pdf}
    \caption{The control graph for creating a foot stall policy.}
    \label{fig:stall}
\end{figure}

\subsection{Foot Juggling with Different Heights}

For the foot juggling skill, we can randomize the desired traveling distance of ball $h$ in the vertical direction to train policy that can be capable of juggling the soccer ball at different heights. See Fig.~\ref{fig:height} for visualization.

\begin{figure}
    \centering
    \includegraphics[width=\columnwidth]{figures/height.pdf}
    \caption{We can generate a foot juggling policy that juggles the ball to different height.}
    \label{fig:height}
\end{figure}
