# Supplementary material for: Hierarchical Planning and Control for Box Loco-Manipulation
Source: arXiv:2306.09532 source file (2023-07-08)
Supplement: Supplementary file 2 [file appendix.tex]

\section{Weight-blended MOE vs Layer-wised MOE}
\label{mann_vs_layer}
\subsection{Equivalency between Weight-blended MOE and Layer-wise MOE}

\edit{
The forward pass of a fully connected neural network with $L$ layers involves the following computations for each layer $l$:
\begin{align*}
    x_l = activation(W_lx_{l-1}),
\end{align*}
where activation is a fixed nonlinear function, $x_0$ is the input, $W_l$ is the learnable matrix at layer $l$. Note that we omit the bias term but it can be included by appending a $1$ to all $x_l$.}
\edit{
For a weight-blended MOE, the computation at each layer will be:
\begin{align*}
    x_l = activation(\sum_g(w_g W_{g, l}) x_{l-1}),
\end{align*}
where $w_g$ and $W_{g,l}$ is the gating weight and the corresponding expert parameters for expert $g$. Since every operation before the activation is linear, this is equivalent to 
\begin{align*}
    x_l = activation(\sum_gw_g (W_{g, l} x_{l-1})),
\end{align*}
where instead of computing the weighted sum of $W_{g,l}$ first, we compute $W_{g,l}x_{l-1}$ independently first and compute the weighted sum of their results. This corresponds to our formulation of layer-wise MOE.
}

\subsection{Computational Efficiency}
\edit{
Even though the weight-blended interpretation and layer-wise MOE interpretation are equivalent, they require dramatically different compute resources. In the weight-blended interpretation, when we desire to perform forward pass or backward pass with a batch of data with batch size $B$, we need to copy all the parameters in $W_{g,l}$ $B$ times in order to perform batch operation. This requires additional memory of $\mathcal{O}(Bmn)$ where $m, n$ are the size of the matrix $W_{g,l}$. On the other hand, layer-wise MOE can perform this operation in the usual manner without additional copying of data. 
}
\edit{
The speed up of layer-wise MOE compared to weight-blended MOE is related to the batch size $B$. When $B$ is small (around 32-64) as in the supervised learning setting, the speedup is around 10x. The speedup grows almost linearly with the batch size. Weight-blended MOE used up all $8GB$ of GPU memory when the batch size reaches 512 and stops working, while layer-wise MOE continues to operate efficiently. In RL, we use large batch size (10000), which is impossible to implement using weight-blended MOE with our hardware setup.
Our layer-wise MOE is inspired by the implementation from~\cite{2020-siggraph-motion_vae}; however, we focus on physics-based motion control, while theirs is kinematic. 
}

\section{Adjacency Matrix for Multiple Skills and Their Transitions}
\label{app:adjacency}
We design many soccer juggling skills and their transitions with our control graph. In Table~\ref{tab:control_graph}, we show the adjacency matrix for this control graph.

\begin{table*}[t]
    \centering
    \small
    \caption{Adjacency matrix for control graph with many skills. $1$ indicates a directed edge going from the row node to the column node.}
    \begin{tabular}{|P{0.04\textwidth}|P{0.04\textwidth}|P{0.04\textwidth}|P{0.04\textwidth}|P{0.04\textwidth}|P{0.04\textwidth}|P{0.04\textwidth}|P{0.04\textwidth}|P{0.04\textwidth}|P{0.04\textwidth}|P{0.04\textwidth}|P{0.04\textwidth}|P{0.04\textwidth}|P{0.04\textwidth}|P{0.04\textwidth}|}
        \hline
         & LFD& LFU & LKD & LKU & LAWD & LAWU & HD & HU & RFD& RFU & RKD & RKU & RAWD & RAWU\\
         \hline
         LFD &  & 1 & &  & & 1& & & & & & & &\\
         \hline
         LFU & 1  & &1 & & & &1 & &1 & &1 & &  &\\
         \hline
         LKD &  & & & 1 & & & & & & & & & &\\ 
         \hline
         LKU &1 & & 1  & & & &1 & &1 & &1 & & &\\
         \hline
         LAWD & & 1& & & & 1 & & & & & & & &\\
         \hline
         LAWU & & & & & 1 & & & & & & & & & \\
         \hline
         HD & & & & & & & & 1 & & & & & &\\
         \hline
         HU  &1 & & 1  & & & &1 & &1 & &1 & & &\\
         \hline
         RFD & & & & & & & & & & 1 & & & & 1\\
         \hline
         RFU &1 & & 1  & & & &1 & &1 & &1 & & &\\
         \hline
         RKD & & & & & & & & & & & & 1 & & \\
         \hline
         RKU &1 & & 1  & & & &1 & &1 & &1 & & & \\
         \hline
         RAWD & & & & & & & & & &  1& & & & 1\\
         \hline
         RAWU & & & & & & & & & & & & & 1 & \\
         \hline
    \end{tabular}
    \label{tab:control_graph}
\end{table*}
